# Supplementary material for: Learning to Factorize and Relight a City
Source: arXiv:2008.02796 source file (2020-08-06)
Supplement: Supplementary file 1 [file supp-fig-rotation.tex]

\begin{figure*}[t]
    \begin{center}
    \includegraphics[width=0.95\linewidth]{./supp_images/rotation_v0.pdf}
    \end{center}
    \caption{We demonstrate our disentangled azimuth representation by showing an input scene with the sun synthesized at different azimuths. Note that shadows are appear and move in a plausible manner.}
    \label{fig:rotation}
\end{figure*}
